# Supplementary material for: Spatio-Temporal Field Neural Networks for Air Quality Inference
Source: arXiv:2403.02354 source file (2024-06-06)
Supplement: Supplementary file 1 [file appendix.tex]

\section{Curl of the Gradient Field}\label{curless prove}
Importantly, the recovered gradients possess real physical significance, manifesting in special properties such as a constant zero-curl, which can be formulated as 
\begin{equation}\label{gradient eq}
    \nabla \times \mathbf{F} = \nabla \times \nabla G = \mathbf{0}
\end{equation}
and it will be theoretically proven in the following:

\begin{theorem}
    $\nabla \times \mathbf{F} = \nabla \times \nabla G = \mathbf{0}$
\end{theorem}
\begin{proof}
Let $f(x,y,z)$ be a scalar-valued function. Then its gradient 
\begin{equation}
    \nabla f(x,y,z)=(\frac{\partial f}{\partial x}(x,y,z), \frac{\partial f}{\partial y}(x,y,z), \frac{\partial f}{\partial z}(x,y,z))
\end{equation}
is a vector field, which we denote by $\mathbf{F}=\nabla f$. We can easily calculate that the curl of $\mathbf{F}$ is zero. We use the formula for curl $\mathbf{F}$ in terms of its components
\begin{equation}
    \text{curl}\text{ }\mathbf{F} = (\frac{\partial F_3}{\partial y}-\frac{\partial F_2}{\partial z}, \frac{\partial F_1}{\partial z}-\frac{\partial F_3}{\partial x}, \frac{\partial F_2}{\partial x}-\frac{\partial F_1}{\partial y}). 
\end{equation}
Since each components of $\mathbf{F}$ is a derivative of $f$, we can rewrite the curl as 
\begin{equation}
    \text{curl}\text{ }\nabla f=(\frac{\partial^2 f}{\partial y \partial z}-\frac{\partial^2 f}{\partial z \partial y}, \frac{\partial^2 f}{\partial z \partial x}-\frac{\partial^2 f}{\partial x \partial z}, \frac{\partial^2 f}{\partial x \partial y}-\frac{\partial^2 f}{\partial y \partial x}).
\end{equation}
If $f$ is twice continuously differentiable, then its second derivatives are independent of the order in which the derivatives are applied. All the terms cancel in the expression for curl $\nabla f$, and we conclude that curl $\nabla f=\textbf{0}$.
\end{proof}

Additionally, we have experimentally demonstrated it in Section \ref{curl experiment}. This property holds substantial importance in accurately characterizing the three-dimensional vectors representing the STF's gradient, enhancing the overall interpretability of our model.

Another way to express Equation (\ref{gradient eq}) is that $\mathbf{F}$ is \textit{conservative}, which means that the result of the curve integration is only dependent on the start and end points of the integration path, and not on the shape of the path itself. For convenience, we set $\mathcal{C}$ to be a straight line from the start to the end.

\section{Addition to Implementation}
\subsection{Implementation of Ring Estimation}\label{ring inference}
% The Ring Estimation module operates on the ring zones. It utilizes $\left[\mathbf{D}_{\cdot,j} \right]_{:K}$ of the outer edge and the coordinates of the transition nodes $\left[\mathbf{c}_{\cdot,j+1}^{tns} \right]_{:K}$ on the inner edge to estimate the $\left[\mathbf{D}_{\cdot,j+1} \right]_{:K}$ of the inner edge. The pseudo-code is shown in Algorithm \ref{ring estimation psu}. In the first operation, $\left[\mathbf{D}_{\cdot,0} \right]_{:K} \in \mathbb{R}^3$ is obtained by concatenating $\mathbf{X}^{src}$ and the encoding of the source node $\mathbf{p}^{src}$, and feed them to a three-layers MLP to compress the dimension to three, as shown in row 3.
The Ring Estimation module operates on ring zones, utilizing outer edge information $\left[\mathbf{D}{\cdot,j} \right]{:K}$ and transition node coordinates $\left[\mathbf{c}{\cdot,j+1}^{tns} \right]{:K}$ to estimate $\left[\mathbf{D}{\cdot,j+1} \right]{:K}$ of the inner edge. Pseudo-code in Algorithm \ref{ring estimation psu} outlines the process. In the first operation, $\left[\mathbf{D}{\cdot,0} \right]{:K} \in \mathbb{R}^3$ is obtained by concatenating $\mathbf{X}^{src}$ and the encoding of the source node $\mathbf{p}^{src}$, compressed to three dimensions using a three-layer MLP (row 3).

Considering that the coding of difference and coordinate of a node are in the same vector space $\mathbb{R}^{10}$, the Transformer-Decoder is a suitable structure for the Ring Estimation as it can capture the correlation between $K$ nodes and utilize information from the last inference. We first use the spatio-temporal encoding module (noted as $STEncoder$) mentioned in Section \ref{st encoding sec} to encode the coordinates of the inner edges and the difference from the outer edges as $\mathbf{P}_{TAR}$ and $\mathbf{P}_{MEM}$, respectively, where $\mathbf{P}_{TAR}\in\mathbb{R}^{K\times10}$ is used as the TARGET input of the Transformer-Decoder (noted as $Decoder1$) and $\mathbf{P}_{MEM}\in\mathbb{R}^{K\times10}$ is used as the MEMORY input (row 9-10). The output of $Decoder1$ is processed to obtain the difference, multiplied by $W_g \in \mathbb{R}^{10\times3}$ after passing through the activation function $GeLU$ (row 11).
% To obtain the difference, we pass the output of $Decoder1$ through an activation function $GeLU$ and multiply it by $W_g \in \mathbb{R}^{10\times3}$ (row 11). 

To obtain the residual $\Delta \mathbf{y}$ between $\hat{\mathbf{Y}}^{tar}$ and $\left[\mathbf{y}_{\cdot}^{src}\right]_{:K}$, we use a queue to store the difference obtained from each operation (row 5). The final $\Delta \mathbf{y}$ is computed by summing up differences and projecting them onto their respective unit direction vectors (row 15). Here, $\vec{\mathbf{R}} = \left[\vec{\mathbf{r}}{\cdot}\right]{:K} \in \mathbb{R}^{K\times3}$ represents the concatenation of all unit direction vectors of neighbors.

% At the end of the loop, we sum up all the differences and obtain $\Delta \mathbf{y}$ by projecting them on their respective unit direction vectors (row 15). Here, $\vec{\mathbf{R}} = \left[\vec{\mathbf{r}}_{\cdot}\right]_{:K} \in \mathbb{R}^{K\times3}$ represents the concatenation of all the unit direction vectors of the neighbors.
% Residuals $\Delta \mathbf{y}$ between $\hat{\mathbf{Y}}^{tar}$ and $\left[\mathbf{y}{\cdot}^{src}\right]{:K}$ are obtained using a queue to store differences from each operation (row 5). 
% Since the Transformer-Decoder is a common structure, due to space constraints, we will present its principle and implementation in detail in the Appendix \ref{trans decoder}, but will not go into it here.

\subsection{Implementation of Neighbor Aggregation}\label{neighbor aggregation implementation}
We use $Decoder2$ to denote the Transformer-Decoder network we utilized in Neighbor Aggregation. In order to make sure that the dimensions of the TARGET and the MEMORY input are the same, we copy the target coordinates $K$ times to make them match the dimensions of the source coordinates, and then we encode them in $\mathbf{P}^{src}\in\mathbb{R}^{K\times10}$, act as the TARGET input, and $\mathbf{P}^{tar}\in\mathbb{R}^{K\times10}$, act as the MEMORY input. To obtain $\mathbf{W}$, we first multiplied the output by $W_N \in \mathbb{R}^{10\times1}$ to transform it into a Logit score. Then, we applied the $Softmax$ operation to ensure that the weights sum up to one. In this end, the formulation of the Neighbor Aggregation can be written as
\begin{equation}
    \mathbf{W} = Softmax\left( W_N \cdot Decoder2(\mathbf{P}^{src}, \mathbf{P}^{tar}) \right)
    % \vspace{-1em}
\end{equation}

\begin{algorithm}[h]
	\caption{Ring Estimation} 
        \textbf{Input}: $\mathbf{C}^{src},\mathbf{X}^{src},\left[\mathbf{y}_{\cdot}^{src}\right]_{:K},\mathbf{C}^{tar}$\\
        \textbf{Output}: $\hat{\mathbf{Y}}^{tar}$
        \begin{algorithmic}[1]
            \STATE $\vec{\mathbf{R}} = \left( \mathbf{C}^{tar}-\mathbf{C}^{src} \right) \big/ \left( \Vert \mathbf{C}^{tar}-\mathbf{C}^{src} 
            \Vert \right)$
            \STATE $\mathbf{P}^{src} = STEncoder\left( \mathbf{C}^{src} \right)$
            \STATE $\left[\mathbf{D}_{\cdot,0} \right]_{:K} = MLP\left( \left[ \mathbf{P}^{src}; \mathbf{X}^{src} \right] \right) $
            \STATE $\mathbf{C}^{start} = \mathbf{c}^{src}$
            % \STATE /*  */
            \STATE grad\_buffer = $\left[ \mathbf{D}_0, \right]$       // \textit{grad\_buffer is a queue}
            % \COMMENT{grad\_buffer is a list}
		\FOR {$j=1,2,\ldots m$}
                \STATE $\left[\mathbf{D}_{\cdot,j-1} \right]_{:K}$ = grad\_buffer$\left[-1\right]$ 
                % \COMMENT{Take the last output}
                \STATE $\mathbf{C}^{end} = \mathbf{C}^{start} + \vec{\mathbf{R}}$
                \STATE $\mathbf{P}_{TAR} = STEncoder\left(\mathbf{C}^{end}\right)$
                \STATE $\mathbf{P}_{MEM} = STEncoder\left(\left[\mathbf{D}_{\cdot,j-1} \right]_{:K}\right)$
			\STATE grad = $W_g\cdot GeLU\left(Decoder1\left(\mathbf{P}_{TAR},\mathbf{P}_{MEM}\right)\right)$
			\STATE grad\_buffer.append(grad)
			\STATE $\mathbf{C}^{start} \leftarrow \mathbf{C}^{end}$
		\ENDFOR
            \STATE $\Delta \mathbf{y} = \vec{\mathbf{R}} \cdot Sum$(grad\_buffer) 
            % \COMMENT{Accumulate the difference}
            \STATE $\hat{\mathbf{Y}}^{tar} = \left[\mathbf{y}_{\cdot}^{src}\right]_{:K} + \Delta \mathbf{y}$
	\end{algorithmic} 
        \label{ring estimation psu}
\end{algorithm}
\vspace{-0.5em}
